# Supplementary material for: Polar Indirect Valley as a Limiting Factor for Radiative Efficiency in Gold-Based Mixed-Valence Double Perovskites
Source: arXiv:2505.01904 source file (2025-05-03)
Supplement: Supplementary file 1 [file Article_polar-valley__SI_VF.pdf]

# **SUPPLEMENTARY INFORMATIONS**

## **Polar Indirect Valley as a Limiting Factor for Radiative Efficiency in Gold-Based Mixed-Valence Double Perovskites.**

*Ange B. Chambissie Kameni<sup>1</sup>, Alexandre Py-Renaudie<sup>1</sup>, Damien Garrot<sup>2</sup>, Baptiste Berenguier<sup>1</sup>, Guillaume Bouchez<sup>2</sup>, Davide Raffaele Ceratti<sup>3</sup>, Philip Schulz<sup>1</sup>, Jean-François Guillemales<sup>1</sup> and Géraud Delport<sup>1\*</sup>.*

<sup>1</sup>CNRS, Institut du Photovoltaïque d'Île de France (IPVF) UMR 9006, 18 Bd Thomas Gobert, 91120 Palaiseau, France

<sup>2</sup> Université Paris-Saclay, UVSQ, CNRS, GEMAC, Versailles, 78000, France

<sup>3</sup> ParisTech-CNRS, PSL Research University, Institut de Recherche de Chimie Paris (IRCP), Paris, France

### **Supplementary section 1: Attribution of the Raman Pics**

In this section, we present the Lorentzian fitting of the Raman modes of the AuClAu compound in the non-resonant configuration. The extracted mode positions are then compared with values reported in the literature<sup>1</sup> for the resonant state, highlighting potential shifts induced by the different excitation conditions.

The following formula was used to fit the two peaks using Lorentzian functions:

$$L(x) = A_1 \cdot \frac{1}{1 + \left(\frac{x - x_1}{\Gamma_1}\right)^2} + A_2 \cdot \frac{1}{1 + \left(\frac{x - x_2}{\Gamma_2}\right)^2}$$

Where  $A_1$  and  $A_2$  are the amplitudes of the peaks,  $\Gamma_1$  and  $\Gamma_2$  the two full widths at half maximum,  $x_1$  and  $x_2$  the central positions.

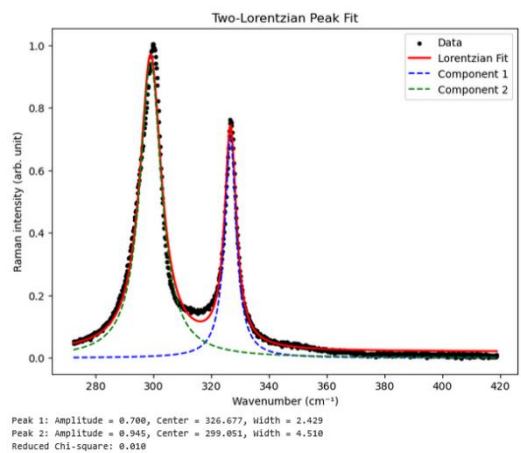

**Figure S1:** Lorentzian fitting of the Raman modes of the AuClAu compound in the non-resonant configuration (excitation at 1,58 eV), with the vibrational modes located at 299 cm<sup>-1</sup> and 326.6 cm<sup>-1</sup>.

| Raman Frequency (cm <sup>-1</sup> ) | Vibration mode      |
|-------------------------------------|---------------------|
| 297                                 | $B_{1g} [AuCl_4^-]$ |
| 299                                 | $A_{1g} [AuCl_4^-]$ |
| 324                                 | $A_{1g} [AuCl_2^-]$ |

**Table S1:** Attribution of the vibration modes from Polarized Resonant Raman taken from the literature<sup>1</sup>

The data analyzed here are derived from pellets (refer to the materials and methods section for details on the synthesis process) consisting of AuClAu powder pressed into a CsCl matrix. The stresses applied during synthesis can alter bond lengths, leading to shifts in vibrational modes. Under applied pressure, the crystal is expected to contract, reducing interatomic bond lengths (particularly between gold and chlorine atoms) and causing the vibrational modes to shift toward higher wavenumbers, as shown in Figure S4. This clarification is provided as a basis for the subsequent analyses of the vibrational mode positions.

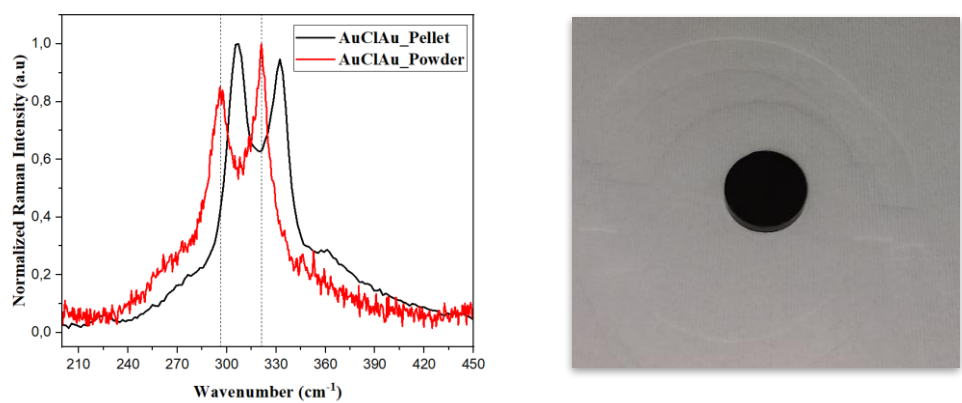

**Figure S2:** a) Resonant Raman spectra comparing the vibration modes in pure powders and pressed powder pellets of AuClAu. The peaks are shifted from 296 cm<sup>-1</sup> to 306 cm<sup>-1</sup> and from 321 cm<sup>-1</sup> to 332 cm<sup>-1</sup>. These shifts are attributed to structural stresses introduced during the pellet synthesis process - b) Image of a pellet of AuClAu after synthesis. The black color of the pellet highlights the highly absorbent nature of the studied material.

## **Supplementary section 2: Band-gap and Urbach-Tail fits**

To compute the value of the direct / indirect bandgap, the Tauc-plot method was applied, involving a linear fit of  $(\alpha(E) * E)^2$  and  $\sqrt{\alpha(E) * E}$  curves respectively<sup>2</sup>.

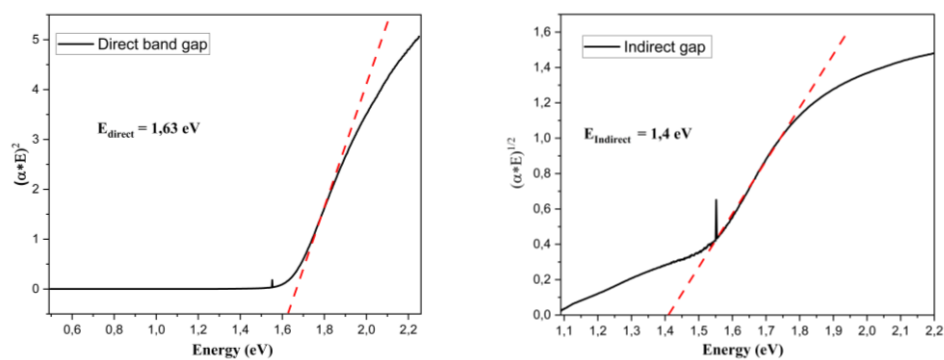

**Figure S3:** a) Direct (1.61 eV) and b) Indirect (1.41 eV) bandgap extraction using the Tauc-plot method. A secondary sub-gap exponential region, corresponding to the Urbach tail, is observed but not included in the fit.

The Urbach component can be determined through a linear fit of the sub-gap region by plotting the absorption curve on a logarithmic scale.

In Figure S4, we present a comparison between PLE spectra and pseudo-absorption spectra at different temperatures. A key observation from these graphs is that, at high energy, the pseudo-absorption saturates while the PLE decreases. This decrease in PLE indicates that non-radiative processes become dominant in this energy range. This behavior is clearly reflected in the RQY discussed in the main text.

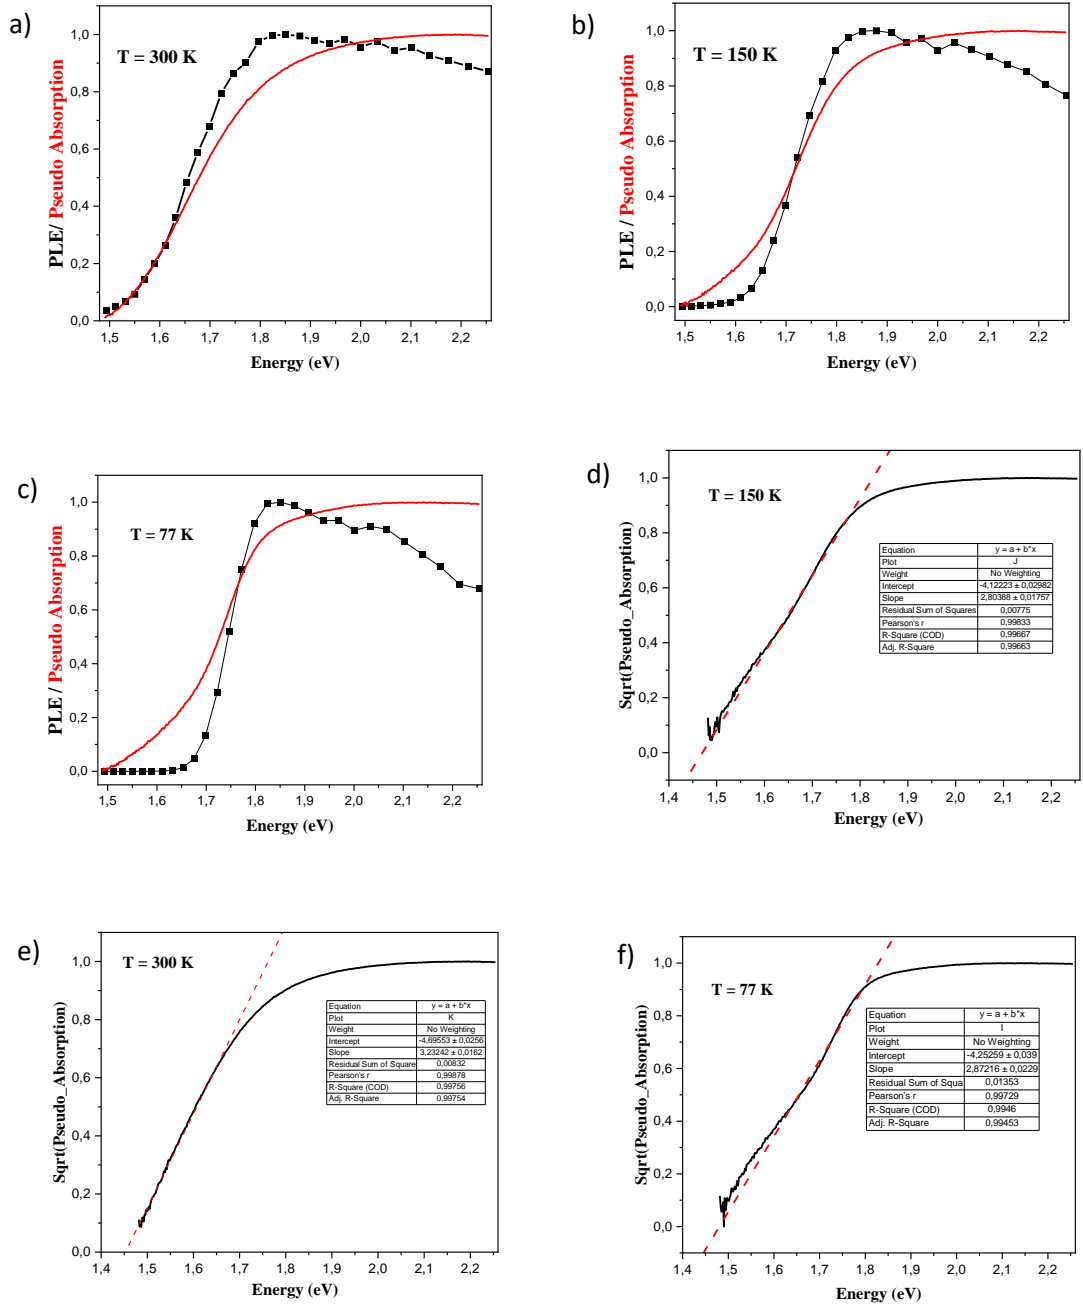

**Figure S4:** (a-c) Comparison between PLE and Pseudo absorption at different temperatures – (d-f) Indirect band gap extraction using the Tauc Plot method.

### **Supplementary section 3:** Estimation of the PLQY using Hyperspectral measurement

The Photoluminescence Quantum Yield (PLQY) is a key parameter that quantifies the luminescence efficiency of a material. In our study, the PLQY of AuClAu was estimated from a photoluminescence measurement, absolutely calibrated in intensity with a BENTHAM white light source. The measurement give access to the PL intensity denotes as  $\Phi_{PL}$  in photons/s/m<sup>2</sup>/sr/J represented in figure S5-a).

The PLQY is defined by the following relation:  $PLQY = \frac{\Phi_{PL}}{\Phi_{Abs}}$

Where  $\Phi_{PL} = \int dS \int d\Omega \cos(\theta) \int dE \Phi_{PL}$  denotes the photon flux emitted via photoluminescence. We assume the emission to be Lambertian, so that  $\Phi_{PL}$  doesn't depend on  $\Omega$ . The integrated spectrum over space is displayed in figure S5-b).

$\Phi_{Abs}$  corresponds to the photon flux absorbed by the sample.

The PL flux is obtained from the measurement  $\Phi_{PL} = \int d\Omega \int dE \Phi_{PL}$ ,

while the absorbed photon flux is given by  $\Phi_{Abs} = (1 - T(h\nu_{laser}) - R(h\nu_{laser})) \frac{I_{laser}}{h\nu_{laser}}$ . Where T and R are respectively the value transmission and the reflexion of the sample at the laser energy.

The dominant uncertainty source here, comes from the measurement made with the powermeter.

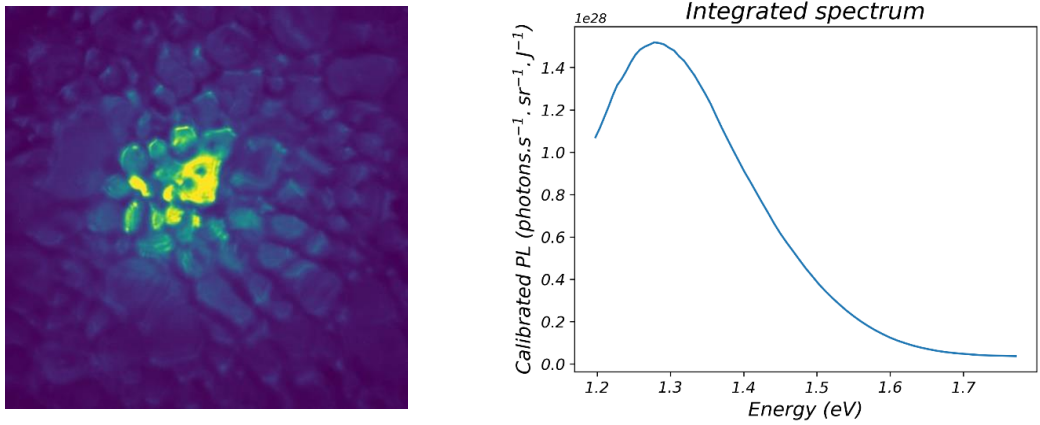

**Figure S5:** a) Broadband photoluminescence (PL) image of the sample acquired with a hyperspectral camera – b) Intensity-calibrated absolute PL spectrum integrated over the entire image shown in (a).

### **Supplementary section 4:** Pseudo Absorption calculation

The evaluation of the pseudo-absorption is based on transmission measurements conducted on AuClAu powder embedded in a CsCl matrix. These measurements are performed as a function of temperature in the range of 300 K to 40 K, on both the Perovskite + CsCl pellet and the reference pellet (CsCl only). The pseudo-absorption is thus determined using the following formula:

$$PseudoAbs = 1 - \frac{T_{(Perovskite+CsCl)}}{T_{(CsCl)}}$$

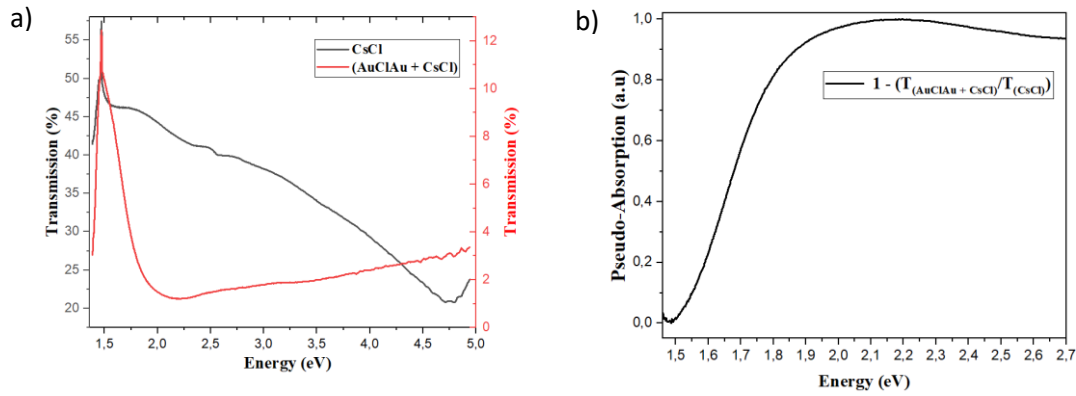

**Figure S6:** a) Transmission of the reference CsCl pellet compared to the transmission of the pellet containing AuClAu powder mixed with CsCl – b) Pseudo-absorption curve derived from the previous transmission measurements.

### **Supplementary section 5:** Time resolved measurements

Figure S7) highlights the Temperature-dependent evolution of the TRPL spectra under 1.91 eV excitation. The inset shows the corresponding carrier lifetimes, revealing that at 300 K it becomes challenging to extract accurate lifetime values due to the proximity with the instrument response function.

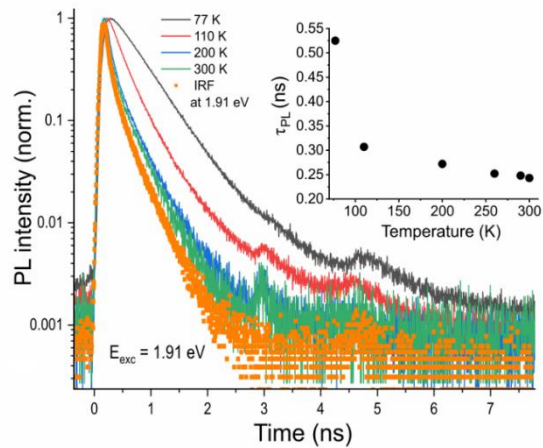

**Figure S7:** TRPL measurements at 1.91 eV as function of temperature and the corresponding lifetime.

Figures S8-a) and S9) respectively show the TRPL measurements and their corresponding fits as a function of temperature, using an excitation energy of 1.65 eV. At this energy, the carrier lifetime remains unchanged with temperature and is effectively equal to the instrument response function (IRF), as if the measurement were directly capturing the IRF itself. This behavior arises because 1.65 eV lies within the polar indirect tail of the absorption spectrum of the AuClAu compound. As discussed in the main text, the measured lifetime corresponds to the time required for carriers to tunnel from the direct to the indirect gap. Therefore, exciting directly within the indirect region has no observable effect, as the carriers are already in this state.

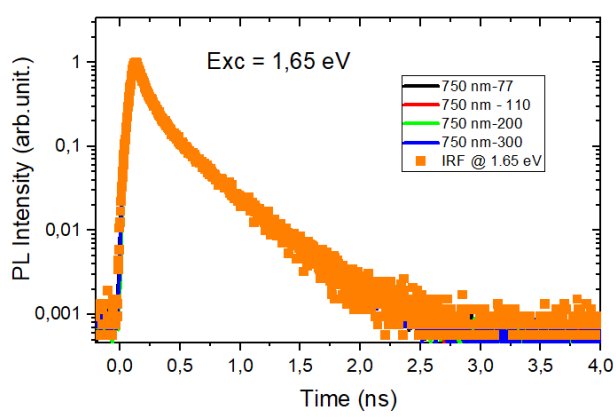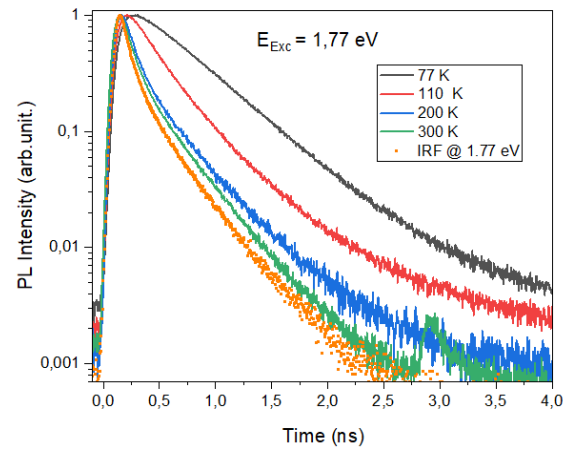

**Figure S8:** TRPL measurements as function of temperature at a) 1.65 eV and b) 1.77 eV excitation laser.

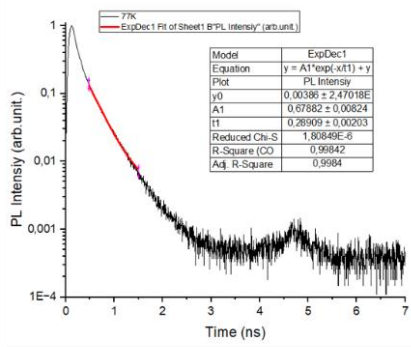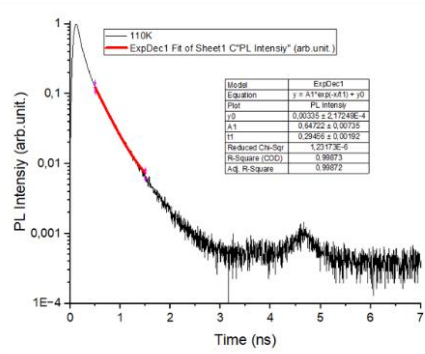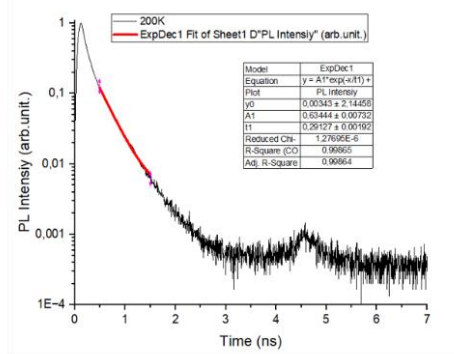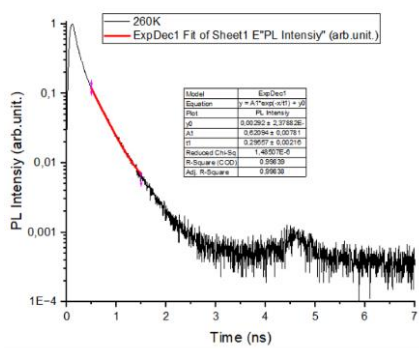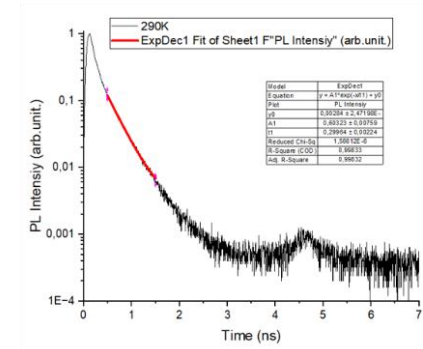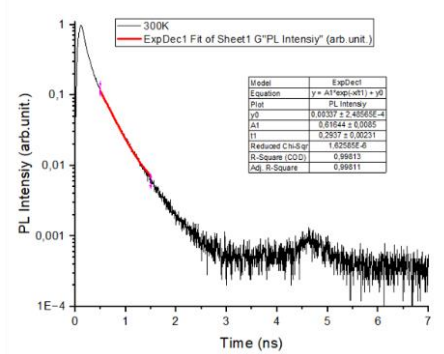

**Figure S9:** Fitting of TRPL (at 1.65 eV) measurements at different temperatures using a mono-exponential decay law, showing a constant carrier lifetime across all temperatures.

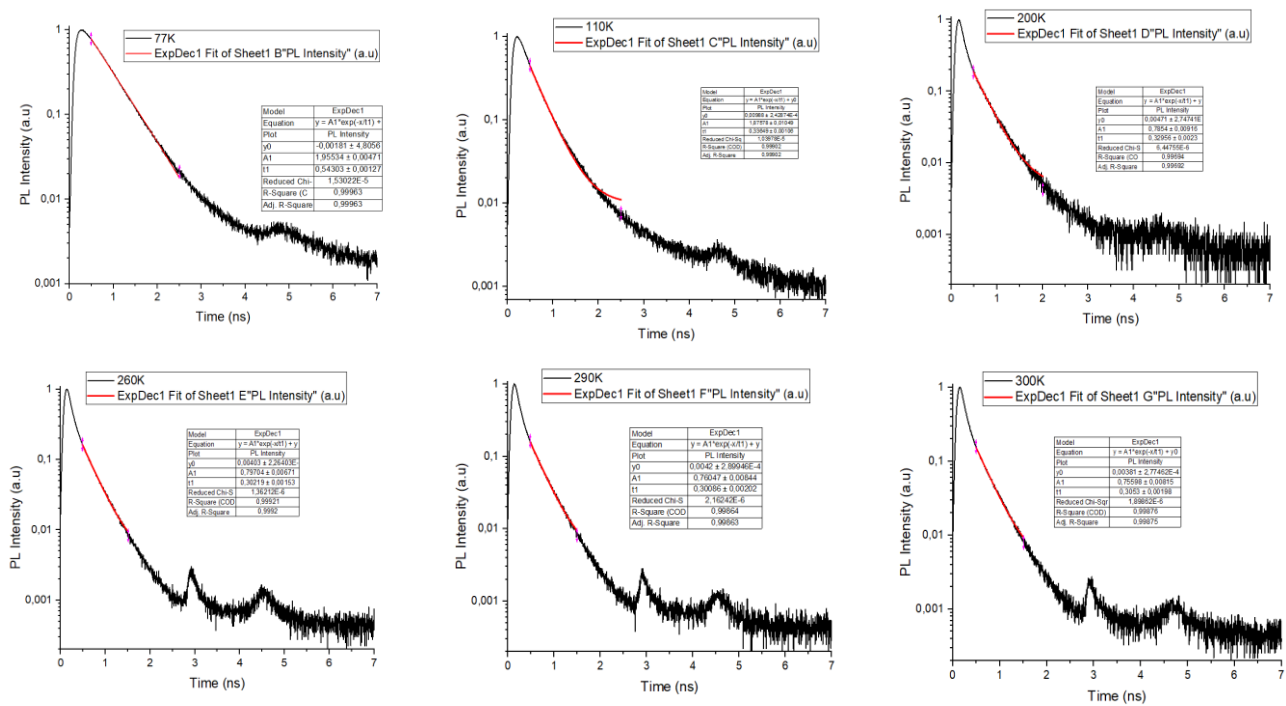

**Figure S10:** Fitting of TRPL (at 1.77 eV) measurements at different temperatures using a mono-exponential decay law, showing a constant carrier lifetime across all temperatures

We also investigated carrier dynamics over longer timescales. Instead of using a short pulse, we employed a 10  $\mu$ s square excitation and monitored the decay. Considering that multiple recombination pathways may exist in the studied compound; we fitted this long-time TRPL with a bi-exponential function. From this fitting, we obtained two characteristic times: a very short one of 0.282  $\mu$ s, which likely corresponds to the time required for carriers to tunnel from the conduction band to the indirect states; and a longer time, consistent with the fact that carriers are now stabilized in the polaronic state described in the main text.

It is important to emphasize that the biexponential function employed in this analysis is purely phenomenological. In typical time-resolved studies of semiconductors, where two characteristic relaxation times are present, the decay dynamics are more rigorously described by a single exponential function with a time-dependent decay rate. In contrast, the use of a simple sum of two independent exponentials, as applied here, does not necessarily reflect the underlying physical processes but serves as a convenient empirical approximation for data fitting.

$$I(t) = A_1 e^{\frac{-t}{\tau_1}} + A_2 e^{\frac{-t}{\tau_2}}$$

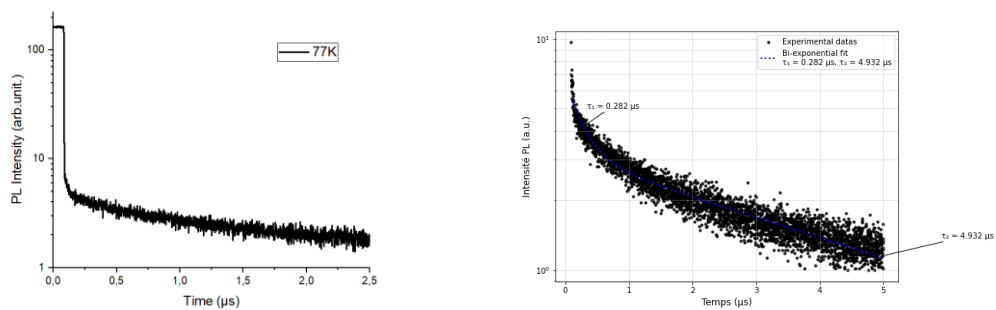

**Figure S11:** (a) Time-resolved photoluminescence (TRPL) measurement over an extended timescale, acquired using a 100 kHz pulsed excitation source (1,9 eV) at 77 K. (b) Bi-exponential fitting applied to the TRPL decay curve to extract the characteristic carrier lifetime

### **Supplementary section 6: Temperature-dependent X-ray diffraction**

Temperature-dependent diffraction measurements were performed to confirm the absence of any phase transitions over the studied range. Figure S illustrates the diffractograms recorded between 80 and 380 K, demonstrating the stability of the tetragonal structure across this temperature range. This observed absence of phase transitions further supports the idea that the optical properties, along with the related polaronic, remain constant with temperature.

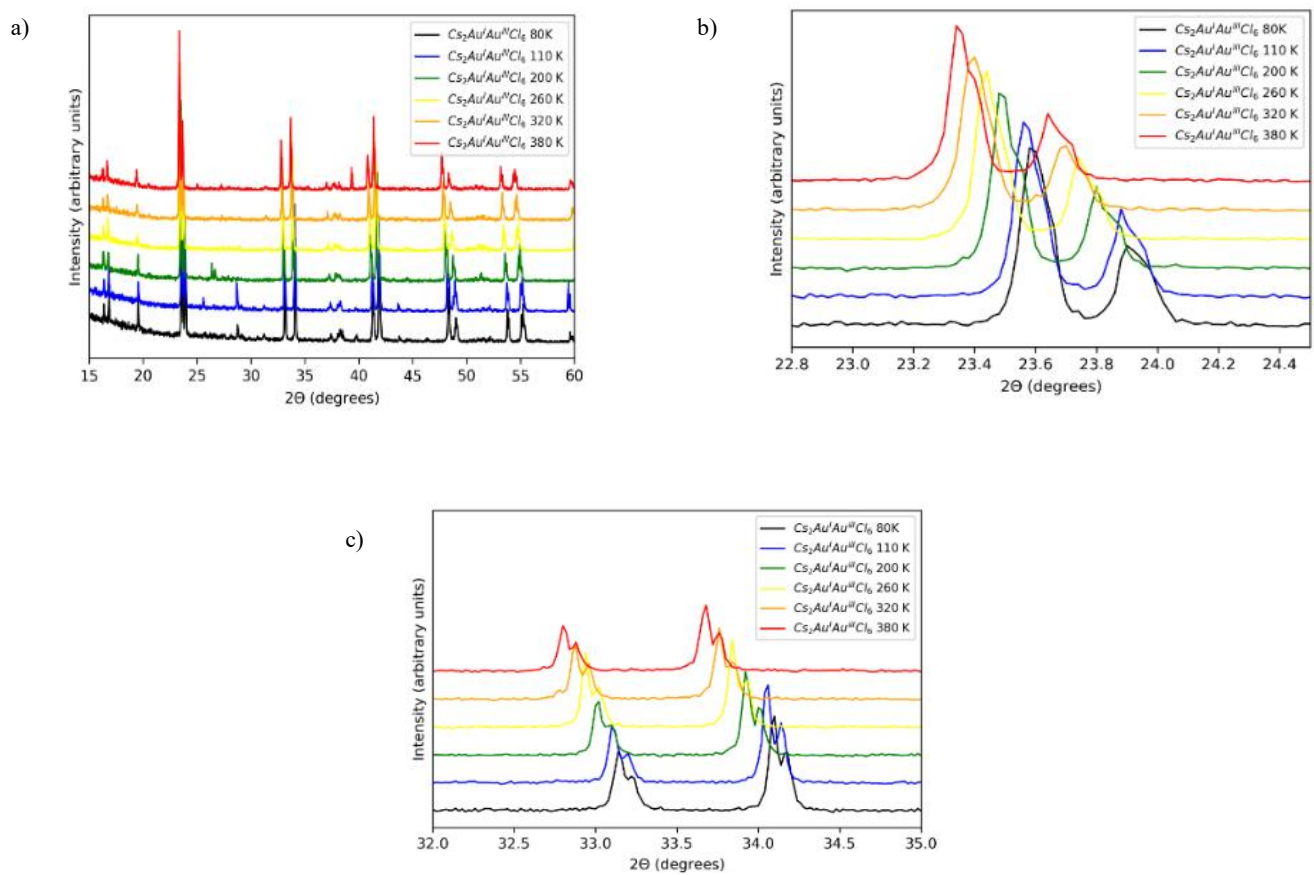

**Figure S12:** a) Powder diffractogram of AuClAu as a function of temperature. No phase transition is detected within this temperature range; only lattice expansion due to heating is observed. b) and c) Enlarged views of the main peaks of the perovskite structure, showing their evolution with temperature.

We also investigated the evolution of the lattice thermal expansion coefficient of these compounds and compared it to that of their lead-based counterparts (especially MAPbCl<sub>3</sub>). As shown in Figure S13), this coefficient is approximately three times higher, indicating that the compound is more prone to structural distortion than the lead-based material in the tetragonal form.

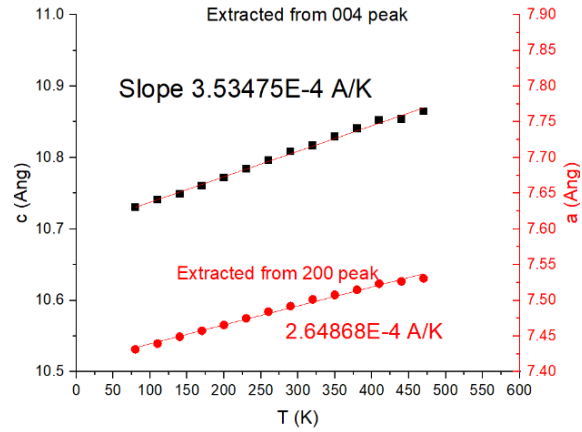

**Figure S13:** Evolution of the lattice parameter extracted from the previous data's of the two main diffraction peaks (004) and (200).

From these values, we can extract the linear thermal expansion coefficient with respect to the a and c lattice parameters using this formula:  $\alpha_L = \frac{1}{L} * \frac{dL}{dT}$ . We then have  $\alpha_a = \frac{3.53475E-4}{10.8} = 3.27292E-5 \text{ K}^{-1}$  and  $\alpha_c = \frac{2.64868E-4}{7.55} = 3.50819E-5 \text{ K}^{-1}$ . These values are of the same order of magnitudes than those obtained in the MAPbCl<sub>3</sub><sup>3</sup> perovskite composition which is  $5.45E-5 \text{ K}^{-1}$ .

#### **Supplementary section 7: PLE measurements**

Excited photoluminescence (PLE) is an optical spectroscopy method used to gain additional insights into the absorption characteristics of a semiconductor material. It relies on the dependence of the material's emission intensity (luminescence) on the excitation energy. Unlike absorption measurements, which probe the states responsible for light absorption, this technique focuses on the states that emit light. By combining both approaches, it is possible to deduce the different energy levels involved in absorption and emission processes within the material. This correspondence is valid only under the assumption that all generated electron-hole pairs recombine radiatively.

For this measurement, we use a pulsed laser with a frequency of 78 MHz, scanning wavelengths from 550 nm to 830 nm with a 10nm bandwidth. Luminescence spectra are measured at each of these wavelengths, and the area under the curve is calculated. The PLE signal is then obtained by normalizing this area to the acquisition time and the number of incident photons (equation 2). Here, we made sure that the number of incident photons was the same for all excitation wavelengths. For the Temperature-dependent measurements, the sample is placed in a cryostat coupled to a liquid nitrogen dewar. The temperature is varied from 300 K to 77 K in steps of 50 K, with a 10-minute wait at each temperature to ensure the sample reaches the target temperature.

$$I_{PL} = C \phi_{photons_{out}}(\nu) = C \eta_{PL} A(\nu) \phi_{photons_{in}}(\nu) \quad (1)$$

$$\frac{I_{PL}}{\phi_{photons_{in}}(\nu)} = C' A(\nu) \quad (2)$$

$$\phi_{photons_{in}}(\nu) = \frac{P_{in}(\nu)}{h\nu} \quad (3)$$

In the main text, we estimated the RQY value. This calculation was performed by taking the ratio between the PLE and the absorption. By considering that the PLE measures the intensity of photons emitted by the sample, dividing it by the absorption allows us to estimate the luminescence efficiency of the sample.

From the PLE measurements we can extract the value of the Urbach energy using a linear fit to estimate the slope of the PLE spectrum in log scale. The formula that we use are the following:

$$PLE \approx \exp\left(\frac{E - E_g}{Eu}\right)$$

$$\ln(PLE) = \frac{1}{Eu} (E - E_g)$$

$$Eu = \frac{1}{slope}$$

In this formula,  $E_g$  represent the pseudo band gap energy.

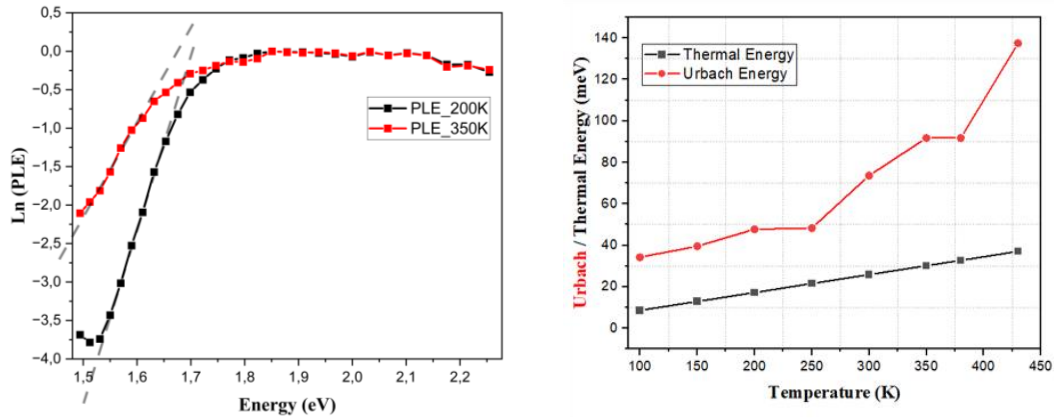

**Figure S14:** Analysis of the Urbach energy. (Left) Linear fit of the slope of the PLE at 200K and 350K in log scale. (Right) Temperature dependence of the Urbach energy extracted from PLE and of the thermal energy.

### **Supplementary section 8: Optimization of the powder dilution**

Given the strong absorption characteristics of this material, a series of dilution experiments were performed by embedding the perovskite powder into a transparent CsCl matrix, with the objective of determining the optimal concentration for accurate optical analysis. Among the tested dilutions, the 0.1% perovskite-to-CsCl ratio emerged as the most appropriate, as it enabled a clear observation of the band edge and enhanced the overall readability of the absorption spectrum. As shown in Figure S15, increasing the perovskite concentration leads to a progressive rise in infrared absorption. This behavior can be attributed to the saturation of absorption in the visible range, making the infrared component more prominent. This observation further supports the notion that, in these materials, there is indeed a significant contribution from electronic states extending into the infrared region.

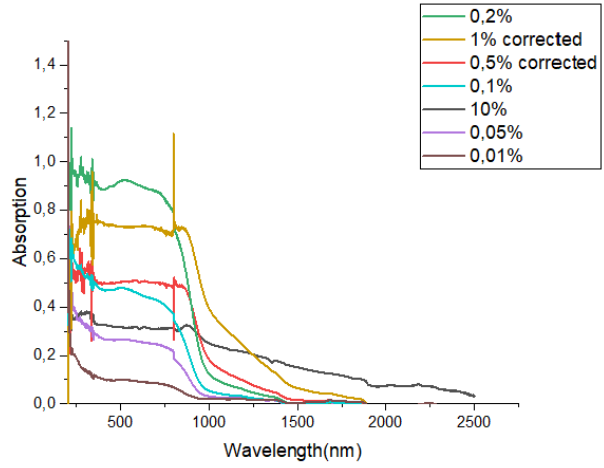

**Figure S15:** Evolution of the absorption spectra as function of the powder dilution in the transparent matrix.

#### **Supplementary section 9: Arrhenius fit of the PL spectrum**

Figure S16 presents a fit of the photoluminescence intensity as a function of temperature using the model given by:

$$I_{PL}(T) = I_{PL}(0) \frac{1}{1 + \exp\left(\frac{-E_A}{K_B T}\right)}$$

$$\ln\left(-1 + \frac{I_{PL}(0)}{I_{PL}(T)}\right) = -E_A \frac{1}{K_B T}$$

The fitted curve is expected to follow a linear relationship, which, in principle, should exhibit no intercept at the origin. However, the experimental data clearly deviate from this expectation, revealing a non-zero intercept. This deviation indicates that the activation energy is not constant over the temperature range investigated. In fact, the activation energy is found to vary with temperature, suggesting that the physical process involved cannot be accurately described using a simple Arrhenius model. Instead, a more advanced formalism that accounts for the thermal dependence of the activation energy is required, as implemented in the main text. This observation further supports the presence of electron–phonon coupling in the system.

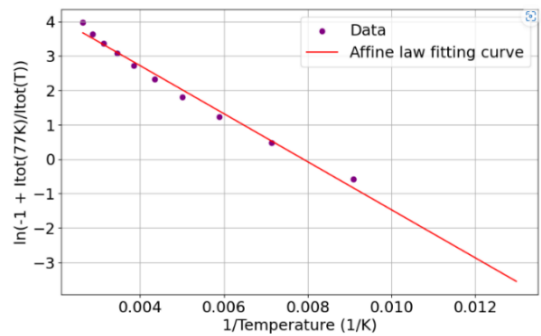

**Figure S16:** Arrhenius fit of the PL intensity as function of the temperature

### **Supplementary section 10 : PL en fonction de l'excitation à 300K**

Here, we present photoluminescence data recorded at 300 K using various excitation wavelengths. No shift in the peak position is observed compared to the spectra obtained at low temperature, indicating that the emission energy remains stable across the investigated excitation conditions.

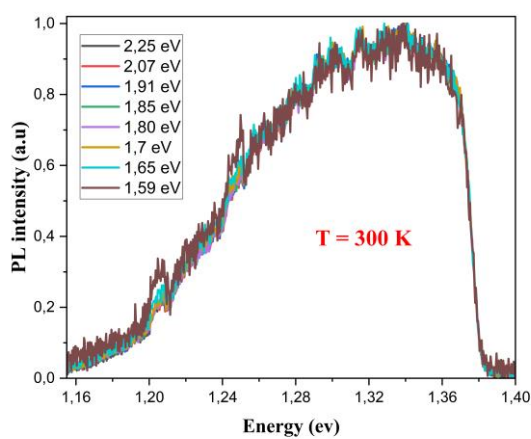

**Figure S17:** Evolution of photoluminescence spectra measured at 300 K under different excitation wavelengths, covering both the direct and indirect absorption regions. Despite the variation in excitation energy, the photoluminescence peak position remains unchanged, indicating that the emission originates from the same radiative recombination pathway.

### **References**

1. Liu, X. J. Pressure-induced phase transition in mixed-valence gold complexes  $\text{Cs}_2\text{Au}_2\text{X}_6$  ( $\text{X}=\text{Cl}$  and  $\text{Br}$ ). *Journal of Chemical Physics* **110**, 9174–9178 (1999).
2. Tauc, J., Grigorovici, R. & Vancu, A. *Optical Properties and Electronic Structure of Ge Optical Properties and Electronic Structure of Amorphous Germanium*. *phys. stat. sol* vol. 15 (1966).
3. Handa, T. *et al.* Large thermal expansion leads to negative thermo-optic coefficient of halide perovskite  $\text{CH}_3\text{NH}_3\text{PbI}_3$ . *Phys Rev Mater* **4**, (2020).
